# Supplementary material for: Overcoming Quadratic Hardware Scaling for a Fully Connected Digital Oscillatory Neural Network
Source: arXiv:2504.20680 source file (2025-04-29)
Supplement: Supplementary file 1 [file 8_appendix.tex]

\section{appendix}
This is the appendix
